# Supplementary material for: Stability (over time) of Modified-CS and LS-CS for Recursive Causal Sparse Reconstruction
Source: arXiv:1006.4818 source file (2010-06-24)
Supplement: Supplementary file 1 [file LSCS_stab_appendix.tex]

\section{Appendix: Complete Proof of LS-CS Stability} %Proof of Theorem \ref{stabres2} and Corollary \ref{stabres2_cor}}% and $\Aset_t$ being disjoint with $\Nhat_{t-1}$
We prove Theorem \ref{stabres2} by induction. First notice that using condition \ref{initass} of the theorem, the result holds for $t=0$. This proves the base case. For the induction step, assume that the result holds at $t-1$, i.e. $\tDelta_{t-1} \subseteq \Sset_{t-1}(d_0)$, and $|\tDelta_{t-1}| \le (2d_0-2)S_a$,  $|\tDelta_{e,t-1}| =0$, $|\tT_{t-1}| \le S_0$. Use this to prove that the result holds for $t$.

Since $T_t = \tT_{t-1}$, so $|T_t| \le S_0$.

Notice that $N_t = N_{t-1} \cup \Aset_t \setminus \Rset_t$, $\Rset_t \subseteq N_{t-1}$ and $\Aset_t \subseteq N_{t-1}^c$. Since $\Delta_{e,t} = \Nhat_{t-1} \setminus N_t =  \Nhat_{t-1} \cap [(N_{t-1}^c \cap \Aset_t^c) \cup \Rset_t] \subseteq \tDelta_{e,t-1} \cup \Rset_t = \Rset_t$. The last equality follows because $|\tDelta_{e,t-1}| =0$. Thus $|\Delta_{e,t}| \le |\Rset_t| = S_a$.

Now, $\Delta_t = N_t \setminus \Nhat_{t-1}  = (N_{t-1} \cap \Nhat_{t-1}^c \cap \Rset_t^c) \cup (\Aset_t \cap \Nhat_{t-1}^c) = (\tDelta_{t-1} \cap  \Rset_t^c) \cup (\Nhat_{t-1}^c \cap \Aset_t)$. Thus, $\Delta_t$ will be largest if $\tDelta_{t-1}$ is largest and is disjoint with $\Rset_t$ (i.e. $\tDelta_{t-1} =\Sset_{t-1}(d_0)$) and $\Nhat_{t-1}$ is disjoint with $\Aset_t$.
Thus, in the worst case, $\Delta_t =(\Sset_{t-1}(d_0)  \cap  \Rset_t^c) \cup \Aset_t$. If $d_0>1$, $\Sset_{t-1}(d_0)$ is not empty, $\Rset_{t} \subseteq \Sset_{t-1}(d_0)$ and $\Aset_t \subseteq \Sset_{t-1}(d_0)^c$, and thus in the worst case, $|\Delta_t| = |\Sset_{t-1}|-|\Rset_t|+|\Aset_t| =(2d_0-2)S_a - S_a + S_a = (2d_0-2)S_a$. If $d_0=1$, $\Delta_t = \Aset_t$ and so $|\Delta_t|=S_a$.
Thus, $|\Delta_t| \le \max(S_a,(2d_0-2)S_a)=k^a$.

% (elements of $\Aset_t \cup (\Sset_{t-1} \cap \Iset_{t-1})$) (elements of $(\Sset_{t-1} \cap \Dset_{t-1}) \setminus \Rset_t$)
%From the above discussion, $\Delta_t \subseteq (\Sset_{t-1}  \cap  \Rset_t^c) \cup \Aset_t$.

From the above discussion, $\Delta_t \subseteq \Sset_{t-1}(d_0) \cup \Aset_t \setminus \Rset_t$. So, in the worst case, $\Delta_t$ contains $S_a$ elements each with magnitudes $M/d, 2M/d \dots d_0M/d$ and $S_a$ elements each with magnitudes $M/d, 2M/d \dots (d_0-2)M/d$.
Consider the detection step at time $t$. Apply Lemma \ref{detectcond} with $S_T = S_0$, $S_\Delta = k^a$, $b= d_0M/d$ and $\gamma=1$. With this choice of $\gamma$, $\Delta_1 \subseteq \Iset_t(d_0)$ and so $|\Delta_1| \le S_a$. Also, $\Delta_2 \subseteq \Sset_t(d_0) \setminus \Dset_t(d_0)$. Thus $\|x_{\Delta_2}\|^2 \le e^2$.
Since conditions \ref{measmodel} and \ref{add_del} hold, all the undetected elements of $\Iset_{t}(d_0)$ will definitely get detected at time $t$. Thus $\tDelta_{\dett,t} \subseteq \Delta_t \setminus \Iset_{t}(d_0) \subseteq \Sset_{t-1}(d_0) \cup \Aset_t \setminus (\Rset_t \cup \Iset_{t}(d_0)) = \Sset_t(d_0) \setminus \Dset_{t}(d_0)$. The last equality follows from (\ref{sseteq}). Thus, $|\Delta_{\dett,t}| \le \max(0,(2d_0-3)S_a)=k^d$.

%$\Delta_{\dett,t} \subseteq \Sset_{t-1} \cup \Aset_t \setminus (\Rset_t \cup \Iset_{d_0,t})$.
%\{i \in \Sset_{t-1}:|x_{t,i}|=d_0M/d\}$. The RHS set is equal to $\Sset_t(d_0) \setminus (\Dset_t \setminus \Dset_{t-1})$. $\Delta_t^c$  with magnitude $d_0 M/d$
%and in the worst case it is equal to %minus the $S_a$ elements with magnitude $d_0M/d$.

 In the detection step, there are at most $f$ false additions (from condition \ref{addthresh}) and thus $|\tDelta_{e,\dett,t}| \le |\Delta_{e,t}| + f \le S_a+f$.

Also, $|\tT_{\dett,t}| \le |N_t| + |\tDelta_{e,\dett,t}| \le S_0+S_a+f$.

%From the earlier discussion, $\tDelta_{\dett,t} \subseteq \Sset_{t-1}(d_0) \cup \Aset_t \setminus (\Rset_t \cup \Iset_{t}(d_0))$. From (\ref{sseteq}), this set is equal to $\Sset_t(d_0) \setminus \Dset_{t}(d_0)$.
Apply Lemma \ref{nofalsedelscond} with $S_T = S_0+S_a+f$, $S_\Delta = k^d$, $b_1 = d_0M/d$, and use the fact that $\tDelta_{\dett,t} \subseteq \Sset_t(d_0) \setminus \Dset_{t}(d_0)$ to bound $\|x_{\tDelta_{\dett}}\|^2$ by $\sm$. Since conditions \ref{measmodel} and \ref{add_del} hold, all elements of $\tT_\dett$ with magnitude greater than or equal to $b_1=d_0 M/d$ will definitely not get falsely deleted. But nothing can be said about the elements of $\Dset_{t}(d_0)$ (or other smaller ones which may have got added) and in the worst case $\tDelta_t$ may contain all of these elements, i.e. it may be equal to $\Sset_t(d_0)$. Thus, $\tDelta_t \subseteq \Sset_t(d_0)$ and so $|\tDelta_t| \le (2d_0-2)S_a$.
%((\Sset_{t-1}  \cap  \Rset_t^c) \cup \Aset_t \setminus \Dset_{d_0,t}) \cup \Dset_t = \Sset_t$.

%\Sset_t$. So, $|\tDelta_t| \le |\Sset_t|=(2d_0-2)S_a$.
%\subseteq \Sset_t(d_0) \setminus (\Dset_t \setminus \Dset_{t-1})$. Notice that $(\Dset_t \setminus \Dset_{t-1})$ contains the $S_a$ elements of $\Dset_t$ with magnitude $(d_0-1)M/d$.

Apply  Lemma \ref{truedelscond} with $S_T = S_0+S_a+f$, $S_\Delta = k^d$ and use $\tDelta_{\dett,t} \subseteq \Sset_t(d_0) \setminus \Dset_{t}(d_0)$ to bound $\|x_{\tDelta_{\dett}}\|^2$ by $\sm$. Since condition \ref{delthresh} holds, all elements of $\tDelta_{e,\dett,t}$ will get deleted by the deletion step. Thus $|\tDelta_{e,t}|=0$.

Also, $|\tT_t| \le |N_t| + |\tDelta_{e,t}| \le S_0$.

This finishes the proof of the induction step and hence of the theorem.%

For the first part of Corollary \ref{stabres2_cor}, apply Theorem \ref{stabres2} to bound $|\tDelta_{t-1}|,|\tT_{t-1}|,|\tDelta_{e,t-1}|$. The discussion above then gives the desired bounds on $|\Delta_t|,|T_t|,|\Delta_{e,t}|$ and $|\tDelta_{\dett,t}|,|\tT_{\dett,t}|,|\tDelta_{e,\dett,t}|$.
The second and third part follow using $\tDelta \subseteq \Sset_t(d_0)$ and $\Delta \subseteq \Sset_{t-1}(d_0) \cup \Aset_t \setminus \Rset_t$.
%The second and third part follow using $\tDelta \subseteq \Sset_t(d_0)$ and $\Delta \subseteq \Sset_t(d_0) \cup \Aset_t$.%and so $\|x_\tDelta\|^2 \le \sm$.%

%For the first part of Corollary \ref{stabres2_cor}, apply Theorem \ref{stabres2} to bound $|\tDelta_{t-1}|,|\tT_{t-1}|,|\tDelta_{e,t-1}|$. The discussion above then gives the desired bounds on $|\Delta_t|,|T_t|,|\Delta_{e,t}|$ and $|\tDelta_{\dett,t}|,|\tT_{\dett,t}|,|\tDelta_{e,\dett,t}|$. %The second and third part follow using $\tDelta \subseteq \Sset_t(d_0)$ and $\Delta \subseteq \Sset_t(d_0) \cup \Aset_t$.%and so $\|x_\tDelta\|^2 \le

%For the first part of the corollary, at any $t > 0$, apply the theorem to obtain the bounds on $|\tDelta_{t-1}|,|\tT_{t-1}|,|\tDelta_{e,t-1}|$. Then use the discussion above to obtain bounds on $|\Delta_t|,|T_t|,|\Delta_{e,t}|$ and $|\tDelta_{\dett,t}|,|\tT_{\dett,t}|,|\tDelta_{e,\dett,t}|$. The second part of the corollary follows easily from the fact that $\tDelta \subseteq \Sset$ and so $\|x_\tDelta\|^2 \le \sm$.
